# Supplementary material for: Transitions, Losses, and Re-parameterizations: Elements of Prediction Games
Source: arXiv:1805.08622 source file (2018-05-20)
Supplement: Supplementary file 1 [file appendix.tex]

% \appendix

%\subsection*{Proper Losses}
%If $\hat{\eta}$ is to be interpreted as an estimate of the true positive class probability $\eta$ then it is desirable to require that $L\br{\eta ,\hat{\eta}}$ be minimised when $\hat{\eta}=\eta$ for all $\eta \in [0,1]$. Losses that satisfy this constraint are said to be \textit{Fisher consistent} and are known as \textit{proper scoring rules} (Buja et al., 2005; Gneiting and Raftery, 2007). To use common machine learning terminology we will refer to Fisher consistent
%losses as \textit{proper losses}. This implies that a proper loss $\ell$ satisfies $\underline{L}\br{\eta} = L\br{\eta,\eta}$ for all $\eta \in [0,1]$.
%
%We will say a loss is \textit{fair} whenever $\eta \mapsto \ell\br{0,\eta}$ and $\eta \mapsto \ell\br{1,\eta}$ are, respectively, right continuous at $0$ and left continuous at $1$, and
%\[
%\ell\br{0,0} = \ell\br{1,1} = 0 .
%\]
%That is, no loss incurred for perfect prediction and there are no sudden ``jumps" in penalty for near-perfect prediction.
%
%We will require that the loss be \textit{definite}, that is, its point-wise Bayes risk at $0$ and $1$ must be bounded from below:
%\[
%\underline{L}\br{0} > -\infty , \underline{L}\br{1} > -\infty .
%\]
%Since properness of a loss ensures $\underline{L}\br{\eta} = L\br{\eta,\eta}$ we see that a fair proper loss is necessarily definite since $L\br{0,0} = \ell\br{0,0} = 0 > -\infty$, and similarly for $L\br{1,1}$. Conversely, if a proper loss is definite then the finite values $\ell\br{0,0}$ and $\ell\br{1,1}$ can be subtracted from $\ell\br{0,\cdot}$ and $\ell\br{1,\cdot}$ to make it fair.
%
%We require a loss to be \textit{regular}, that is,
%\[
%\lim_{\eta \searrow 0}{\eta \ell\br{1,\eta}} = \lim_{\eta \nearrow 1}{(1-\eta) \ell\br{0,\eta}} = 0 .
%\]
%Intuitively, this condition ensures that making mistakes on events that never happen should not incur a penalty. It is not difficult to show that any fair, definite loss is also regular (thus, a proper and fair loss is also regular) but the converse does not hold.
%
%Recall that if $\cS \subseteq \bR^d$ is a convex set, then a convex function $\phi : \cS \rightarrow \bR$ defines a \textit{Bregman divergence}
%\[
%B_\phi\br{s, s_0} := \phi\br{s} − \phi\br{s_0} − \ip{s-s_0}{\nabla \phi\br{s_0}} .
%\]
%When $\cS = [0,1]$, the concavity of $\underline{L}$ means $\phi\br{s} = -\underline{L}\br{s}$ is convex and so induces the Bregman divergence
%\[
%B_\phi\br{s, s_0} := -\underline{L}\br{s} + \underline{L}\br{s_0} − (s_0-s) \underline{L}'\br{s_0} = L\br{s,s_0} - \underline{L}\br{s}
%\]
%by Theorem~\ref{proper-char}. The converse also holds. Given a Bregman divergence $B_\phi$ over $\cS = [0,1]$ the convexity of $\phi$ guarantees that $\underline{L} = -\phi$ is concave. Thus, we know that there is a proper loss $\ell$ with Bayes
%risk equal to $-\phi$. As noted by Buja et al. (2005, sec19), the difference
%\[
%B_\phi\br{\eta,\hat{\eta}} = L\br{\eta,\hat{\eta}} - \underline{L}\br{\eta}
%\]
%is also known as the \textit{point-wise regret} of the estimate $\hat{\eta}$ w.r.t. $\eta$. The corresponding \textit{(full) regret} is the $M$-average point-wise regret
%\[
%\Ee{X\sim M}{B_\phi\br{\eta\br{X},\hat{\eta}\br{X}}} = \bL\br{\eta,\hat{\eta},M} - \underline{\bL}\br{\eta,M} .
%\]


%\subsection*{Graphical Representations}

%Risk curves are closely related to the \textit{cost curves} of Drummond and Holte (2006) as well as idealised \textit{receiver operating characteristic, or ROC curves} (Fawcett, 2004). Proposition ?? makes this latter relationship explicit via a point-line duality between risk and ROC curves. Additionally, results about the Neyman-Pearson function by Torgersen (1981) allow us to establish a transformation
%between suitably smooth maximal ROC and minimal risk curves.



%\subsection*{Risk Curves}
%
%\begin{figure}
%	\centering
%	\begin{tikzpicture}
%	\begin{axis}[domain=0:1, xlabel={$c$}, ylabel={$\bL_c$}, axis x line=bottom, axis y line=left, ymin=0, ymax=0.275, xmin=0, xmax=1.15, xtick={0,0.5,1}, ytick={0.25}]
%	\addplot[color=gray,dashed] (0,0)--(0.5,0.25);
%	\addplot[color=gray,dashed] (0.5,0.25)--(1,0);
%	\draw [black] (0.55,0.23) node[right] {$\underline{\bL}_c\br{\pi}$};
%	
%	\draw [thick, black] plot [smooth, tension=0.7] coordinates { (0,0) (0.25,0.0825) (0.45,0.0725) (0.6,0.0745) (0.8,0.0675) (1,0)};
%	\draw [black] (0.35,0.0845) node[above] {$\bL_c \br{\eta,\hat{\eta}}$};
%	
%	\draw [thick, gray!50] plot [smooth, tension=0.8] coordinates { (0,0) (0.5,0.0625) (1,0)};
%	\draw [black] (0.8,0.0305) node[left] {$\underline{\bL}_c\br{\eta}$};
%	
%	\end{axis}
%	\end{tikzpicture}
%	\caption{Example of a risk curve for costs diagram showing risk curves for costs for the true posterior probability $\eta$ (bottom, grey curve), an estimate $\hat{\eta}$ (middle, bold curve) and the majority class or prior estimate (top, dashed curve).\label{risk-figure}}
%\end{figure}
%
%Risk curves are a graphical representation closely related to ROC curves that take into account a prior $\pi$ in addition to the binary experiment $(P,Q)$. They provide a concise summary of the risk of an estimator $\hat{\eta}$ for the full range of costs $c \in [0,1]$ for a fixed prior $\pi \in [0,1]$, or, alternatively, for the full range of priors $\pi$ given a fixed cost $c$.
%
%A \textit{risk curve for costs} for the estimator $\hat{\eta}$ is the set $\bc{\br{c,\bL_c \br{\hat{\eta},\pi,P,Q}} : c \in [0,1]}$ of points
%parameterised by cost. A \textit{risk curve for priors} for the estimator $\hat{\eta}$ is the set $\bc{\br{\pi,\bL^{0-1} \br{\hat{\eta},\pi,P,Q}} : \pi \in [0,1]}$.
%
%Figure~\ref{risk-figure} shows an example of a risk curve diagram. On it is plotted the cost curves for an estimate $\hat{\eta}$ of a true posterior $\eta$ on the same graph. The ``tent'' function also shown is the risk curve for the majority class predictor $\min\bc{(1-\pi)c, (1-c)\pi}$. Here $\pi = \frac{1}{2}$. Other choices of $\pi \in (0,1)$ skew the tent and the curves under it towards $0$ or $1$.
%
%The weight function $w(c)$ associated with a loss $\ell$ can be interpreted as a weighting on the horizontal axis of a risk curve diagram. When the area under a risk curve is computed with respect to this weighting the result is the full risk $\bL$ since $\bL\br{\eta,\hat{\eta}} = \int_{0}^{1}{\bL_c\br{\eta,\hat{\eta}} w(c) dc}$.
%
%Furthermore, the weighted area between the risk curves for an estimate $\hat{\eta}$ and the true posterior $\eta$ is the regret $\bL\br{\eta,\hat{\eta}} - \underline{\bL}\br{\eta}$ and the statistical information $\Delta \underline{\bL}\br{\eta , M} = \underline{\bL}\br{\pi , M} - \underline{\bL}\br{\eta , M}$ is the weighted area between the ``tent'' risk curve for $\pi$ and the risk curve for $\eta$.
%
%\begin{proposition}
%For a given point $(\mathrm{FP},\mathrm{TP})$ on an ROC diagram the corresponding line in a risk diagram is
%\[
%\bL_c = (1-\pi) c \mathrm{FP} + \pi (1-c) (1- \mathrm{TP}), c \in [0,1]
%\]
%Conversely, the line in ROC space corresponding to a point $(c,\bL_c)$ in risk space is
%\[
%\mathrm{TP} = \frac{(1-\pi) c}{\pi (1-c)} \mathrm{FP} + \frac{(1-\pi) c - \bL_c}{\pi (1-c)} , \, \mathrm{FP} \in [0,1] .
%\]
%\end{proposition}
%
%As mentioned earlier, the Neyman-Pearson lemma guarantees the ROC curve for $\eta$ is maximal. This corresponds to the cost curve being minimal. In fact, these relationships are dual in the sense that there exists a transformation from one to the other as we shall now show.
%
%\begin{theorem}
%	Let $\beta\br{\alpha,P,Q}$ be the Neyman-Pearson function for the binary experiment $(P,Q)$ and 	let $\underline{\bL}\br{\pi,P,Q}$ be the $0-1$ Bayes risk on the same experiment for the prior $\pi$. Then, for any choice of
%	$\pi \in [0,1]$ we have
%	\[
%	\underline{\bL}\br{\pi,P,Q} = \underline{\bL} = \min_{\alpha \in [0,1]}{(1-\pi) \alpha + \pi \br{1-\beta\br{\alpha,P,Q}}} .
%	\]
%	and conversely for any $\alpha \in [0,1]$,
%	\[
%	\beta\br{\alpha,P,Q} = \inf_{\pi \in \left( 0,1 \right]}{\frac{1}{\pi} \br{(1-\pi)\alpha + \pi - \underline{\bL}\br{\pi,P,Q}}}
%	\]
%\end{theorem}
%
%\begin{lemma}
%Suppose $\cX$ contains a connected component $\cC$. Let $\phi: [0,1] \rightarrow [0,1]$ be an arbitrary function that is concave and continuous on $\left( 0,1 \right]$ such that $\phi(1) = 1$. Then there exists distributions $P$ and $Q$ on $\cX$ such that $\beta\br{\alpha,P,Q} = \phi\br{\alpha}$ for all $\alpha \in [0,1]$.	
%\end{lemma}
%
%
%\begin{corollary}
%Suppose $\cX$ contains a connected component. Let $\psi : [0,1] \rightarrow [0,1]$ be an arbitrary concave function such that for all $\pi \in [0,1]$, $0 \leq \psi\br{\pi} \leq \pi \wedge (1-\pi)$. Then there exists distributions $P$ and $Q$ on $\cX$ such that $\underline{\bL}\br{\pi,P,Q} = \psi\br{\pi}$ for all $\pi \in [0,1]$.	
%\end{corollary}
%
%The corollary shows that reasoning about cost-weighted risks for all possible binary experiments $(P,Q)$ can be done purely geometrically. Each experiment can be associated with a concave curve and \textit{vice versa} so that the existence of an experiment becomes equivalent to the existence of a concave curve with certain properties.
%
%******************* Mark's paper *******************************************




%\section{Prediction Problems}


%To do so, the decision maker specifies a function $f \in \hat{Y}^X$, that should have low expected loss,
%\[
%\Ee{(x,y) \sim P}{\ell\br{y,f(x)}} ,
%\]
%where $\ell:Y \times \hat{Y} \rightarrow \bR$ is a loss function that measures the suitability of a prediction $\hat{y}$. Note $Y$ and $\hat{Y}$ need not be the same set, for example in conditional probability estimation $\hat{Y}=\cP\br{Y}$. If $P$ is known to the decision maker, then this is a problem of optimization. In general $P$ is unknown, but the decision maker has access to a sample $S$ of $n$ iid draws from $P$, $\bc{\br{x_i,y_i}}_{i=1}^{n}$. The sample is used as a proxy for expectation under $Y$, and the decision maker returns the function in a restricted class $\cF \subseteq \hat{Y}^X$,


%This is known as the empirical risk minimization (ERM) rule \cite{vapnik1998statistical}. Of central interest are bounds on the \textit{expected loss} of the ERM rule,
%\[
%\Ee{S \sim P^n}{\Ee{(x,y) \sim P}{\ell\br{y,f_S (x)}}}
%\]
%that hold \textit{regardless} of the true value of $P$. What is \textit{unknown} to the decision maker is the distribution $P$. The decision maker acts by specifying a function $f \in \hat{Y}^X$. The loss incurred to the decision maker is the expected predictive performance of $f$. The assumption that the sample is comprised of iid draws from $P$ can be seen as an experiment $e \in \bT\br{\cP\br{X \times Y},\br{X \times Y}^n}$, that maps each distribution to its n-fold product. The ERM rule can be understood as a particular learning algorithm. The risk
%for any learning algorithm $A$ is,
%\[
%\cR_L \br{P,e,A} = \Ee{S \sim P^n}{\Ee{f \sim A\br{S}}{\Ee{(x,y) \sim P}{\ell\br{y,f (x)}}}}.
%\]
%Requiring that the risk is small for all $P$ is then exactly a requirement that the minimax risk of $A$ is small.
%
%For the remainder of the thesis we focus on prediction problems for general experiments, where the decision maker is given access to data that is not of the form of iid draws from $P$.

%Example: Supervised Learning
%\begin{center}
%	\supervisedlearningtask
%\end{center}

%Many suitable losses exists but normally $L(\theta,a)$ is the misclassification probability of the classifier $a$ when used against the distribution $\theta$.
%For instance, the worst-case ratio of output relative entropy to input relative entropy for all possible pairs of input distributions is bounded from above by unity, by the data processing theorem. However, for a fixed reference input distribution, this quantity may be strictly smaller than one, giving so-called strong data processing inequalities (SDPIs). The same considerations apply to an arbitrary $f$-divergence.
%
%The well-known data processing inequality for the relative entropy states that, for any two probability distributions $\mu,\nu$ over an alphabet $\cX$ and for any stochastic transformation (channel) $T$ with input alphabet $\cX$ and output alphabet $\cY$,
%\[
%\bI\br{T \circ \nu , T \circ \mu} \leq \bI\br{\nu , \mu} ,
%\]
%where $T \circ \mu$ denotes the distribution at the output of $T$ when the input has distribution $\mu$ (and similarly for $T \circ \nu$). However, if we fix the reference distribution $\mu$ and vary only $\nu$, then in many cases it is possible to show that $\bI\br{T \circ \nu , T \circ \mu}$ is strictly smaller than $\bI\br{\nu , \mu}$ unless $\nu \equiv \mu$. To capture this effect, we define the quantity
%\[
%\eta\br{\mu , T} := \sup_{\nu \neq \mu}{\frac{\bI\br{T \circ \nu , T \circ \mu}}{\bI\br{\nu , \mu}}} ,
%\]
%and we say that the channel $T$ satisfies a strong data processing inequality (SDPI) at input distribution $\mu$ if $\eta\br{\mu , T} < 1$. In a remarkable paper \cite{ahlswede1976spreading}, Ahlswede and G$\acute{a}$cs have uncovered deep relationships between $\eta\br{\mu , T}$ and several other quantities, such as the maximal correlation and so-called hypercontractivity constants of a certain Markov operator associated to the pair $\br{\mu , T}$. For example, they have shown that if $\cX = \cY = \bc{0, 1}$, $\mu = \text{Bern}(1/2)$,
%and $T = \text{BSC}(\epsilon)$, then $\eta\br{\mu , T}=(1-2 \epsilon)^2$, which is also equal to the squared maximal correlation in the joint distribution $P_{XY}$ with $P_X = P_Y = \text{Bern}(1/2)$ and $P_{Y \mid X} = \text{BSC}(\epsilon)$, the so-called doubly symmetric binary source (DSBS) with parameter $\epsilon$.
%
%After the pioneering work of Ahlswede and G$\acute{a}$cs, the contraction properties of relative entropy (and other $f$-divergences \cite{liese2006divergences}) under the action of stochastic transformations have been studied by several other authors \citep{cohen1993relative,choi1994equivalence,cohen1998comparisons,del2003contraction}. In particular, Cohen et al. \cite{cohen1993relative}, who were the first ones to take up this subject after \cite{ahlswede1976spreading}, showed that the SDPI constant of any channel $T$ with respect to any $f$-divergence is always upper-bounded by the so-called \textit{Dobrushin contraction coefficient} of $T$ \citep{dobrushin1956central,dobrushin1956central2}, another well-known numerical measure of the amount of noise introduced by a channel. 

%An important class of $f$-divergences arises in the context of Bayesian estimation. Given a parameter $\eta \in \br{0,1}$, consider a random pair $\br{\Theta , X}$ with
%\[
%\Theta \sim \text{Bern} \br{\eta} \text{  and  } P_{X \mid \Theta = \theta} = \begin{cases}
%\nu , & \text{ if } \theta = 0\\
%\mu , & \text{ if } \theta = 1 
%\end{cases} .
%\]
%
%Fix an action space $\cA$ and a loss function $\ell : \bc{0, 1} \times \cA \rightarrow \bR$ - in other words, if $\Theta = \theta$ and an
%action $a \in \cA$ is selected, then we incur the loss of $\ell\br{\theta , a}$. Consider the problem of selecting an action in $\cA$ based on some observation $Z$ related to $(\Theta, X)$ via the Markov chain $\Theta \rightarrow X \rightarrow Z$ - i.e., $Z$ and $\Theta$ are conditionally independent given $X$. If $A = \gamma (Z)$ for some function $\gamma$, then we incur the average loss
%\[
%\E{\ell\br{\Theta , \gamma \br{Z}}} = (1-\eta) \E{\ell\br{0 , \gamma \br{Z}}} + \eta \E{\ell\br{1 , \gamma \br{Z}}} .
%\]
%The goal is to pick $\gamma$ to minimize this expected loss for a given observation channel $P_{Z \mid X}$. In the extreme case when $Z$ is independent of $X$, the best we can do is to take
%\[
%a^\star = \argmin_{a \in \cA} \bs{(1-\eta) \ell\br{0 , a} + \eta \ell\br{1 , a}} ,
%\]
%giving us the average loss of
%\[
%L_{\eta}^\star := \inf_{a \in \cA} \bs{(1-\eta) \ell\br{0 , a} + \eta \ell\br{1 , a}} . 
%\]
%On the other hand, if $Z = X$, then we can attain the \textit{minimum Bayes risk}
%\begin{align*}
%	L_{\eta}^\star \br{\nu , \mu} ~:=~& \inf_{\gamma}{\E{\ell\br{\Theta , \gamma \br{X}}}} \\
%	~=~& \inf_{\gamma} \bc{(1-\eta) \int_{\cX}^{}{\ell\br{0,\gamma\br{x}} \nu\br{dx}} + \eta \int_{\cX}^{}{\ell\br{1,\gamma\br{x}} \mu\br{dx}}} ,
%\end{align*}
%where the infimum is over all measurable functions $\gamma : \cX \rightarrow \cA$. 
%\begin{remark}
%	Theorem~\ref{contract-tv-theorem} says that any channel $T$ with $\vartheta \br{T} < 1$ satisfies an SDPI for any $f \in \cF$ at any reference input distribution $\mu \in \cP\br{\cX}$. However, the bounds it gives are generally loose. For example, for $T = \text{BSC}(\epsilon)$ with $\epsilon \in (0, 1)$, we have $\vartheta \br{T} = \card{1 - 2 \epsilon} < 1$, so by Theorem~\ref{contract-tv-theorem}
%	\[
%	\eta_f \br{\text{Bern}(p) , \text{Bern}(\epsilon)} \leq \card{1 - 2 \epsilon} < 1
%	\]
%	for all $f \in \cF$ and all $p \in [0, 1]$. However, as we know from \cite{ahlswede1976spreading},
%	\[
%	\eta \br{\text{Bern}(1/2) , \text{Bern}(\epsilon)} = (1 - 2 \epsilon)^2 < \card{1 - 2 \epsilon} .
%	\]
%\end{remark}

%For any pair $(\mu , T) \in \cP (X) \times \cM (Y \mid X)$, the \textit{maximal correlation} is defined as
%\[
%S (\mu , T) := \sup_{f,g}{\E{f(X) g(Y)}} ,
%\]
%where $(X,Y) \sim \mu \otimes T$, and the supremum is over all $f \in \cF(X), g \in \cF(Y)$ satisfying $\E{f(X)} = \E{g(Y)} = 0$ and $\E{f^2 (X)} = \E{g^2 (Y)} = 1$ (see \cite{witsenhausen1975sequences} and the references therein).

%\subsection{Bounds via maximal correlation}

%Examples (\cite{bhatia2013matrix}):
%\begin{itemize}
%	\item $\Phi (u) = u \log u$ is operator convex.
%	\item $\Phi (u) = u^p$ is operator convex if and only if $p \in [−1, 0] \cup [1, 2]$.
%	\item $\Phi (u) = - u^p$ is operator convex for $0 \leq p \leq 1$.
%\end{itemize}
%In general, it is not easy to determine whether a given function is operator convex. 

%operator convex functions possess very special integral representations:
%\begin{theorem}
%	A function $\Phi : \bR_+ \rightarrow \bR$ with $\Phi (0) = 0$ is operator convex if and only if there exist some constants $\alpha \in \bR , \beta \geq 0$ and a positive measure $v$ on $\bR_+$ satisfying $\int_{0}^{\infty}{(1+t^2)^{-1} v(dt)} < \infty$, such that
%	\[
%	\Phi (u) = \alpha u + \beta u^2 + \int_{0}^{\infty}{\br{\frac{t u}{1+t^2} - \frac{u}{u + t}} v(dt)} .
%	\]
%\end{theorem}
%
%Let $S^2 \br{T} = \sup_{\mu \in \cP\br{\cX}}{ S^2 \br{\mu , T}}$.
%\begin{theorem}
%	\label{operator-contract-theo}
%	Suppose that $\Phi \in \cF$ is operator convex. Then
%	\[
%	\eta_{\Phi} \br{T} = S^2 \br{T} 
%	\]
%	for any discrete channel $T$.
%\end{theorem}

%The data-processing inequality, that is, $I (U;Y) \leq I (U;X)$ for a Markov chain $U \rightarrow X \rightarrow Y$ has been the method of choice for proving impossibility (converse) results in information theory and many other disciplines. Various channel-dependent improvements (called strong data-processing inequalities, or SDPIs) of this inequality have been proposed both classically and more recently.
%Upon passing through a non-degenerate noisy channel distributions become strictly closer and this leads to a loss of information.

%Suppose that estimators are allowed to take values in $A \supseteq \Theta$ and that the loss function is of the form $\ell \br{\rho}$ where $\rho$ is a metric on $\cA$ and
%$\ell : \left[ 0,\infty \right) \rightarrow \left[ 0,\infty \right)$ is a nondecreasing function. The minimax risk for this problem is defined by
%\[
%R := \inf_{\hat{\theta}} \sup_{\theta \in \Theta} \Ee{\theta}{\ell\br{\rho\br{\theta , \hat{\theta}\br{X}}}} ,
%\]
%where the infimum is over all measurable functions $\hat{\theta} : \cX \rightarrow \cA$ and the expectation is taken under the assumption that $X$ is distributed according to $P_\theta$.

%More specifically, one considers a finite subset $\cF$ of the parameter space $\Theta$ and a real number $\eta$ such that $\rho\br{\theta , \theta'} \geq \eta$ for $\theta , \theta' \in \cF , \theta \neq \theta'$ and employs the inequality $R \geq \ell \br{\eta / 2} r$, where
%\[
%r := \inf_{T} \sup_{\theta \in \cF} P_\theta \bc{T \neq \theta} ,
%\]
%the infimum being over all estimators $T$ taking values in $\cF$.
%
%The next step is to note that $r$ is bounded from below by Bayes risks. Let $w$ be a probability measure on $\cF$. The Bayes risk $\bar{r}_w$ corresponding to the prior $w$ is defined by
%\[
%\bar{r}_w := \inf_T \sum_{\theta \in \cF}^{}{w_\theta P_\theta \bc{T \neq \theta}} ,
%\]
%where $w_\theta := w \bc{\theta}$ and the infimum is over all estimators $T$ taking values in $\cF$. When $w$ is the discrete uniform probability measure on $\cF$, we simply write $\bar{r}$ for $\bar{r}_w$. The trivial inequality $r \geq \bar{r}_w$ implies that lower bounds for $\bar{r}_w$ are automatically lower bounds for $r$.


%The space $\Theta$ in which the parameter $\theta \br{P}$ takes values depends on the underlying statistical problem; as an example, if the goal is to estimate the univariate mean $\theta \br{P} = \Ee{P}{X}$, we have $\Theta \subset \bR$. To evaluate the quality of an estimator $\hat{\theta}$, we let $\rho : \Theta \times \Theta \rightarrow \bR_+$ denote a (semi)metric on the space $\Theta$, which we use to measure the error of an estimator for the parameter $\theta$, and let $\Phi : \bR_+ \rightarrow \bR_+$ be a non-decreasing function with $\Phi \br{0} = 0$ (for example, $\Phi \br{t} = t^2$).

%For a given estimator $\hat{\theta}$ - a measurable function $\hat{\theta} : \cX^n \rightarrow \Theta$ - we assess the quality of the estimate $\hat{\theta}\br{X_1,...,X_n}$ in terms of the risk
%\[
%\Ee{P}{\Phi\br{\rho\br{\hat{\theta}\br{X_1,...,X_n} , \theta\br{P}}}} .
%\]

%We use two types of testing problems: one a multiple hypothesis test, the second based on multiple binary hypothesis tests, though we defer discussion of the second.
%
%Given an index set $\cV$ of finite cardinality, consider a family of distributions $\bc{P_v}_{v \in \cV}$ contained within $\cP$. This family induces a collection of parameters $\bc{\theta\br{P_v}}_{v \in \cV}$; we call the family a 2$\delta$-packing
%in the $\rho$-semimetric if
%\[
%\rho \br{\theta\br{P_v} , \theta\br{P_{v'}}} \geq 2 \delta \quad \text{for all } v \neq v' .
%\]
%We use this family to define the \textit{canonical hypothesis testing problem}:
%\begin{itemize}
%	\item first, nature chooses $V$ according to the uniform distribution over $\cV$;
%	\item second, conditioned on the choice $V = v$, the random sample $X = X_1^n = \br{X_1,...,X_n}$ is drawn from the $n$-fold product distribution $P_v^n$.
%\end{itemize}
%Given the observed sample $X$, the goal is to determine the value of the underlying index $v$. We refer to any measurable mapping $\Psi : \cX^n \rightarrow \cV$ as a test function. Its associated error probability is $\P{\Psi\br{X_1^n} \neq V}$, where $\bP$ denotes the joint distribution over the random index $V$ and $X$. In
%particular, if we set $\bar{P} = \frac{1}{\card{\cV}} \sum_{v \in \cV}^{}{P_v}$ to be the mixture distribution, then the sample $X$ is drawn (marginally) from $\bar{P}$, and our hypothesis testing problem is to determine the randomly chosen index $V$ given a sample from this mixture $\bar{P}$.
%
%With this setup, we obtain the classical reduction from estimation to testing.
%
%\begin{proposition}
%	The minimax error has lower bound
%	\[
%	\mathfrak{M}_n \br{\theta\br{\cP}, \Phi \circ \rho} \geq \Phi\br{\delta} \inf_{\Psi}{\P{\Psi\br{X_1^n} \neq V}} ,
%	\]
%	where the infimum ranges over all testing functions.
%\end{proposition}

%Suppose that we have a Bayesian hypothesis testing problem where $V$ is chosen with equal probability to be $1$ or $2$, and given $V = v$, the sample $X$ is drawn from the distribution $P_v$. Denoting by $\bP$ the joint distribution of $V$ and $X$, we have for any test $\Psi : \cX \rightarrow \bc{1,2}$ that the probability of error is
%\[
%\P{\Psi\br{X} \neq V} = \frac{1}{2} P_1 \br{\Psi\br{X} \neq 1} + \frac{1}{2} P_2 \br{\Psi\br{X} \neq 2} .
%\]
%
%\begin{proposition}
%	For any distributions $P_1$ and $P_2$ on $\cX$, we have
%	\[
%	\inf_{\Psi}{P_1 \br{\Psi\br{X} \neq 1} + P_2 \br{\Psi\br{X} \neq 2}} = 1 - \norm{P_1 - P_2}_{\mathrm{TV}} ,
%	\]
%	where the infimum is taken over all tests $\Psi : \cX \rightarrow \bc{1,2}$.
%\end{proposition}

%\begin{theorem}[Assouad’s lemma]
%	Suppose that $\Theta = \bc{0, 1}^d$ and consider the Hamming metric
%	\[
%	\rho_H \br{\theta , \theta'} := \sum_{i=1}^{d}{\ind{\theta_i \neq \theta'_i}} .
%	\]
%	Then
%	\[
%	\mathfrak{M} \br{\Theta} \geq \frac{d}{2} \br{1 - \max_{\theta , \theta' : \rho_H \br{\theta , \theta'} = 1}{\norm{P_\theta - P_{\theta'}}_{\mathrm{TV}}}} .
%	\]
%\end{theorem}

%\cite{scott2012calibrated} -
%Let $\br{X,Y}$ have distribution $P$ on $\cX \times \bc{-1,1}$. Let $\cF$ denote the set of all measurable functions $f: \cX \rightarrow \bc{-1,1}$. Every $f \in \cF$ defines a classifier by the rule $x \mapsto \text{sign}\br{f(x)}$, and in this context $f$ is called a decision function. We adopt the convention $\text{sign}\br{0} = -1$. A loss for binary classification is a measurable function $L : \bc{-1, 1} \times \bR \rightarrow \left[0, \infty \right)$. Any loss can be written
%\[
%L (y, t) = \ind{y=1} L_1 (t) + \ind{y=−1} L_{-1} (t).
%\]
%We refer to $L_1$ and $L_{-1}$ as the partial losses of $L$. The $L$-risk of $f$ is $R_L (f) := \Ee{X,Y}{L \br{Y , f(X)}}$. The optimal $L$-risk is $R_L^\star := \inf_{f \in \cF}{R_L (f)}$.

% 
%
%The cost-sensitive classification loss with cost parameter $\alpha \in (0,1)$ is
%\[
%U_\alpha (y, t) := (1 − \alpha) \ind{y=1} \ind{t \leq 0} + \alpha \ind{y=-1} \ind{t > 0} .
%\]
%
%Define the conditional $L$-risk
%\[
%C_L (\eta , t) := \eta L_1 (t) + (1 - \eta) L_{-1} (t)
%\]
%for $\eta \in [0,1], t \in \bR$, and the optimal conditional $L$-risk $C_L^\star (\eta) = \inf_{t \in \bR}{C_L (\eta , t)}$ for $\eta \in [0,1]$.

%A standard way of evaluating the quality of binary classifiers is by looking at their probability of classification error. Thus, for a classifier $f$ we define the $classification loss (or risk)$
%\[
%L_P (f) := \P{f(X) \neq Y} \equiv \int_{\cX \times \bc{0,1}}^{}{\ind{f(x) \neq y} P\br{dx,dy}} .
%\]
%What is the best classifier for a given P? The answer is given by the following
%\begin{proposition}
%	Given the joint distribution $P$ on $\cX \times \bc{0,1}$, let $\eta \br{x} := \E{Y \mid X=x} \equiv \P{Y=1 \mid X=x}$. Then the classifier
%	\begin{equation}
%		\label{bayes-classfier}
%		f_P^\star \br{x} := \begin{cases}
%			1 , & \text{ if } \eta \br{x} \geq 1/2 \\
%			0 , & \text{ otherwise } 
%		\end{cases}
%	\end{equation}
%	minimizes the probability of classification error over all $f : \cX \rightarrow \bc{0, 1}$, i.e.,
%	\[
%	L_P (f_P^\star) = \min_{f : \cX \rightarrow \bc{0, 1}}{L_P (f)} .
%	\]
%\end{proposition}
%
%The function $\eta$ defined above is called the \textit{regression function}, the classifier in \eqref{bayes-classfier} is called the \textit{Bayes classifier}, and its risk
%\[
%L_P^\star := L_P (f_P^\star)
%\]
%is called the \textit{Bayes rate}.



%\section{Loss, Regret, Conditional Risk and Full Risk}
%***************************************************************
%
%The quality of the composite relation $A \circ \varepsilon: \Theta \rightsquigarrow \cA$ is measured by a loss function $\ell: \Theta \times \cA \rightarrow \bR$. A detailed review of loss functions is given in the next section. The general learning task can more compactly be represented as the pair $(\ell,\varepsilon)$ where $\cA,\Theta,\cX$ can be inferred from the type signatures of $\ell$ and $\varepsilon$. 
%
%\textcolor{red}{We need to incorporate our new notation system here in careful generic manner. If you're going to use regret inside the risk, then you need to draw the reader's attention to the non-standard use of risk.}
%
%We usually encounter the loss relative to the best action defined formally as the \textit{regret} 
%\[
%\Delta \ell \br{\theta,a} := \ell \br{\theta,a} - \inf_{a' \in \cA}{\ell \br{\theta,a'}} .
%\] 
%The quality of the final action chosen by the decision maker when
%they use the decision rule $A$ can be evaluated using the notion of \textit{risk}:
%\[
%\cR_\ell\br{\theta,\varepsilon,A} := \Ee{z \sim \varepsilon (\theta)}{\Ee{a \sim A(z)}{\Delta \ell (\theta, a)}}.
%\]
%which is a function of $\theta$. Two main approaches to find the best decision rule are:
%\begin{itemize}
%	\item Bayesian approach (average case analysis), which is more appropriate if the decision maker has some intuition about $\theta$, given in the form of a prior probability distribution $\pi$, and
%	\item Minimax approach (worst case analysis), which is more appropriate if the decision maker has no prior knowledge concerning $\theta$.
%\end{itemize}
%The Bayesian and max risks are defined as,
%\[
%\cR_{\ell}^\pi \br{\varepsilon,A} := \Ee{\theta \sim \pi}{\cR_\ell \br{\theta,\varepsilon,A}} \text{ and } \cR_\ell \br{\varepsilon,A} := \sup_{\theta \in \Theta}{\cR_\ell \br{\theta,\varepsilon,A}} ,
%\]
%respectively. We measure the difficulty of the general learning task by the \textit{minimum Bayesian risk} and \textit{minimax risk} defined as,
%\[
%\underline{\cR}_{\ell}^\pi \br{\varepsilon} := \min_{A} \cR_{\ell}^\pi \br{\varepsilon,A} \text{ and } \underline{\cR}_{\ell} \br{\varepsilon} := \min_{A} \cR_\ell \br{\varepsilon,A}
%\]
%respectively. 
%
%By using the minimax theorem (\cite{komiya1988elementary}) and finiteness assumptions \textcolor{red}{(Why do the assumptions of the theorem hold - you have made no assumptions on $\ell$)} about $\Theta$ and $\cX$, we obtain the following result that relates the minimum Bayes risk and the minimax risk.
%\begin{theorem}
%	For all experiments $\varepsilon$ and loss functions $\ell$,
%	\[
%	\underline{\cR}_\ell \br{\varepsilon} = \sup_{\pi \in \cP\br{\Theta}}{\underline{\cR}_{\ell}^\pi \br{\varepsilon}} .
%	\]
%\end{theorem}
%
%For any experiment $\varepsilon:\Theta \rightsquigarrow \cX$ we define the \textit{replicated experiment} $\varepsilon_n: \Theta \rightsquigarrow \cX^n$, $n \in \bZ^{+}$, with $\varepsilon_n\br{\theta} = \varepsilon\br{\theta}^n$ the $n$-fold Cartesian product of $\varepsilon\br{\theta}$.
%Usually we wish evaluate the performance of the learning algorithm based on the replicated experiment (which corresponds to obtaining an $n$-sample \textcolor{red}{- bob is not sure of this. to discuss}), thus our main quantity of interest would be $\underline{\cR}_\ell (\varepsilon_n)$.
%
%***************************************************************


%\section{Multi-Class Probability Estimation ($\Theta = \cA = [n]$)}

%\paragraph*{Regret:}
%\begin{align*}
%\textcolor{blue}{\Delta \ell : [n] \times [n] \ni \br{y,\hat{y}} ~\mapsto~}& \textcolor{blue}{\Delta \ell \br{y,\hat{y}} := \ell \br{y,\hat{y}} - \inf_{y' \in [n]}{\ell \br{y,y'}} \in \bR_+} \\
%\Delta \ell : [n] \times \Delta^n \ni \br{y,q} ~\mapsto~& \Delta \ell \br{y,q} := \Ee{\textsf{Y} \sim q}{\textcolor{blue}{\Delta \ell \br{y,\textsf{Y}}}} \in \bR_+ \\ 
%\textcolor{orange}{\Delta \tilde{\ell} : [n] \times \Deltatil^n \ni \br{y,\tilde{q}} ~\mapsto~}& \textcolor{orange}{\Delta \tilde{\ell} \br{y,\tilde{q}} := \textcolor{black}{\Delta \ell \br{y,\Pi_\Delta^{-1}\br{\tilde{q}}}} \in \bR_+} \\
%\textcolor{red}{\Delta \ell : \Delta^n \ni q ~\mapsto~}& \textcolor{red}{\Delta \ell \br{q} := \br{\Delta \ell_1 \br{q},\dots,\Delta \ell_n \br{q}}^\top \in \bR_+^n} \\
%\textcolor{violet}{\Delta \tilde{\ell} : \Deltatil^n \ni \tilde{q} ~\mapsto~}& \textcolor{violet}{\Delta \tilde{\ell} \br{\tilde{q}} := \Pi_\Delta \br{\textcolor{red}{\Delta \ell \br{\Pi_\Delta^{-1}\br{\tilde{q}}}}} \in \bR_+^{n-1}}
%\end{align*}
%where $\textcolor{red}{\Delta \ell_i \br{q} := \textcolor{black}{\Delta \ell \br{i,q}} \in \bR_+ , \, \forall i \in [n]}$. Note that for a \textit{fair} loss $\inf_{y' \in [n]}{\ell \br{y,y'}} = 0$, thus we have $\ell = \Delta \ell$. 

%Let $\tilde{\pi} = \Pi_\Delta \br{\pi} \in \Deltatil^n$ and $\tilde{\eta} = \Pi_\Delta \br{\eta} \in \br{\Deltatil^n}^\cX$.

%\paragraph*{Full Risk, Full Bayes Risk, and Minimum Full Bayes Risk $\br{\pi,\varepsilon}$:}
%
%
%\begin{align*}
%\textcolor{cyan}{\cR_{\textcolor{black}{\ell}} : [n] \times \cM\br{[n],\cX} \times \br{\Delta^n}^\cX \ni \br{y,\varepsilon,q} ~\mapsto~}& \textcolor{cyan}{\cR_{\textcolor{black}{\ell}} \br{y,\varepsilon,q} := \Ee{\textsf{X} \sim \varepsilon\br{y}}{\textcolor{black}{\ell \br{y,q\br{\textsf{X}}}}} \in \bR_+} \\
%\cR_{\ell} : \Delta^n \times \cM\br{[n],\cX} \times \br{\Delta^n}^\cX \ni \br{\pi,\varepsilon,q} ~\mapsto~& \cR_{\ell} \br{\pi,\varepsilon,q} := \Ee{\textsf{Y} \sim \pi}{\textcolor{cyan}{\cR_{\textcolor{black}{\ell}} \br{\textsf{Y},\varepsilon,q}}} \in \bR_+ \\
%\underline{\cR}_{\ell} : \Delta^n \times \cM\br{[n],\cX} \ni \br{\pi,\varepsilon} ~\mapsto~& \underline{\cR}_{\ell} \br{\pi,\varepsilon} := \inf_{q \in \br{\Delta^n}^\cX}{\cR_{\ell} \br{\pi,\varepsilon,q}} \in \bR_+ \\
%\textcolor{cyan}{\cR_{\textcolor{orange}{\tilde{\ell}}} : [n] \times \cM\br{[n],\cX} \times \br{\Deltatil^n}^\cX \ni \br{y,\varepsilon,\tilde{q}} ~\mapsto~}& \textcolor{cyan}{\cR_{\textcolor{orange}{\tilde{\ell}}} \br{y,\varepsilon,\tilde{q}} := \Ee{\textsf{X} \sim \varepsilon\br{y}}{\textcolor{orange}{\tilde{\ell} \br{y,\tilde{q}\br{\textsf{X}}}}} \in \bR_+} \\
%\textcolor{orange}{\cR_{\tilde{\ell}} : \Deltatil^n \times \cM\br{[n],\cX} \times \br{\Deltatil^n}^\cX \ni \br{\tilde{\pi},\varepsilon,\tilde{q}} ~\mapsto~}& \textcolor{orange}{\cR_{\tilde{\ell}} \br{\tilde{\pi},\varepsilon,\tilde{q}} := \Ee{\textsf{Y} \sim \Pi_\Delta^{-1} \br{\tilde{\pi}}}{\textcolor{cyan}{\cR_{\textcolor{orange}{\tilde{\ell}}} \br{\textsf{Y},\varepsilon,\tilde{q}}}} \in \bR_+} \\
%\textcolor{orange}{\underline{\cR}_{\tilde{\ell}} : \Deltatil^n \times \cM\br{[n],\cX} \ni \br{\tilde{\pi},\varepsilon} ~\mapsto~}& \textcolor{orange}{\underline{\cR}_{\tilde{\ell}} \br{\tilde{\pi},\varepsilon} := \inf_{\tilde{q} \in \br{\Deltatil^n}^\cX}{\cR_{\tilde{\ell}} \br{\tilde{\pi},\varepsilon,\tilde{q}}} \in \bR_+} \\
%%%%%%%%%%%%%%%%%%%%%%%%%%%%%%%%%%%%%%%%%%%%%%%%%%%%%%%
%\textcolor{cyan}{\cR_{\textcolor{red}{\ell}} : \cM\br{[n],\cX} \times \br{\Delta^n}^\cX \ni \br{\varepsilon,q} ~\mapsto~}& \textcolor{cyan}{\cR_{\textcolor{red}{\ell}} \br{\varepsilon,q} := \bc{\cR_{\textcolor{red}{\ell_1}} \br{\varepsilon,q},\dots,\cR_{\textcolor{red}{\ell_n}} \br{\varepsilon,q}}^\top \in \bR_+^n} \\
%\textcolor{red}{\cR_{\ell} : \Delta^n \times \cM\br{[n],\cX} \times \br{\Delta^n}^\cX \ni \br{\pi,\varepsilon,q} ~\mapsto~}& \textcolor{red}{\cR_{\ell} \br{\pi,\varepsilon,q} := \pi^\top \cdot \textcolor{cyan}{\cR_{\textcolor{red}{\ell}} \br{\varepsilon,q}} \in \bR_+} \\
%\textcolor{red}{\underline{\cR}_{\ell} : \Delta^n \times \cM\br{[n],\cX} \ni \br{\pi,\varepsilon} ~\mapsto~}& \textcolor{red}{\underline{\cR}_{\ell} \br{\pi,\varepsilon} := \inf_{q \in \br{\Delta^n}^\cX}{\cR_{\ell} \br{\pi,\varepsilon,q}} \in \bR_+} \\
%\textcolor{cyan}{\cR_{\textcolor{violet}{\tilde{\ell}}} : \cM\br{[n],\cX} \times \br{\Deltatil^n}^\cX \ni \br{\varepsilon,\tilde{q}} ~\mapsto~}& \textcolor{cyan}{\cR_{\textcolor{violet}{\tilde{\ell}}} \br{\varepsilon,\tilde{q}} := \Pi_\Delta \br{\cR_{\textcolor{red}{\ell}} \br{\varepsilon,\Pi_\Delta^{-1}\br{\tilde{q}}}} \in \bR_+^{n-1}} \\
%\textcolor{violet}{\cR_{\tilde{\ell}} : \Deltatil^n \times \cM\br{[n],\cX} \times \br{\Deltatil^n}^\cX \ni \br{\tilde{\pi},\varepsilon,\tilde{q}} ~\mapsto~}& \textcolor{violet}{\cR_{\tilde{\ell}} \br{\tilde{\pi},\varepsilon,\tilde{q}} := \Pi_\Delta^{-1}\br{\tilde{\pi}}^\top \cdot \textcolor{cyan}{\cR_{\textcolor{red}{\ell}} \br{\varepsilon,\Pi_\Delta^{-1}\br{\tilde{q}}}} \in \bR_+} \\
%\textcolor{violet}{\underline{\cR}_{\tilde{\ell}} : \Deltatil^n \times \cM\br{[n],\cX} \ni \br{\tilde{\pi},\varepsilon} ~\mapsto~}& \textcolor{violet}{\underline{\cR}_{\tilde{\ell}} \br{\tilde{\pi},\varepsilon} := \inf_{\tilde{q} \in \br{\Deltatil^n}^\cX}{\cR_{\tilde{\ell}} \br{\tilde{\pi},\varepsilon,\tilde{q}}} \in \bR_+} 
%\end{align*}
%where $\textcolor{cyan}{\cR_{\textcolor{red}{\ell_i}} \br{\varepsilon,q} := \cR_{\textcolor{black}{\ell}} \br{i,\varepsilon,q}  \in \bR_+ , \, \forall i \in [n]}$.
%
%\paragraph*{Full Bayes Risk and Minimum Full Bayes Risk $\br{M,\eta}$:}
%\begin{align*}
%\hat{\cR}_{\ell} : \cP\br{\cX} \times \br{\Delta^n}^\cX \times \br{\Delta^n}^\cX \ni \br{M,\eta,q} ~\mapsto~& \hat{\cR}_{\ell} \br{M,\eta,q} := \Ee{\textsf{X} \sim M}{\Ee{\textsf{Y} \sim \eta\br{\textsf{X}}}{\ell\br{\textsf{Y},q\br{\textsf{X}}}}} \in \bR_+ \\
%\underline{\hat{\cR}}_{\ell} : \cP\br{\cX} \times \br{\Delta^n}^\cX \ni \br{M,\eta} ~\mapsto~& \underline{\hat{\cR}}_{\ell} \br{M,\eta} := \inf_{q \in \br{\Delta^n}^\cX}{\hat{\cR}_{\ell} \br{M,\eta,q}} \in \bR_+ \\
%%%%%%%%%%%%%%%%%%%%%%%%%%%%%%%%%%%
%\textcolor{orange}{\hat{\cR}_{\tilde{\ell}} : \cP\br{\cX} \times \br{\Deltatil^n}^\cX \times \br{\Deltatil^n}^\cX \ni \br{M,\tilde{\eta},\tilde{q}} ~\mapsto~}& \textcolor{orange}{\hat{\cR}_{\tilde{\ell}} \br{M,\tilde{\eta},\tilde{q}} := \Ee{\textsf{X} \sim M}{\Ee{\textsf{Y} \sim \Pi_\Delta^{-1}\br{\tilde{\eta}\br{\textsf{X}}}}{\tilde{\ell}\br{\textsf{Y},\tilde{q}\br{\textsf{X}}}}} \in \bR_+} \\
%\textcolor{orange}{\underline{\hat{\cR}}_{\tilde{\ell}} : \cP\br{\cX} \times \br{\Deltatil^n}^\cX \ni \br{M,\tilde{\eta}} ~\mapsto~}& \textcolor{orange}{\underline{\hat{\cR}}_{\tilde{\ell}} \br{M,\tilde{\eta}} := \inf_{q \in \br{\Deltatil^n}^\cX}{\hat{\cR}_{\tilde{\ell}} \br{M,\tilde{\eta},\tilde{q}}} \in \bR_+} 
%\end{align*}
%At this point we note the following facts:
%\begin{itemize}
%	\item Since $\Ee{\br{\textsf{Y} , \textsf{X}} \sim D}{\ell\br{\textsf{Y},q\br{\textsf{X}}}} = \Ee{\textsf{X} \sim M}{\Ee{\textsf{Y} \sim \eta\br{\textsf{X}}}{\ell\br{\textsf{Y},q\br{\textsf{X}}}}} = \Ee{\textsf{Y} \sim \pi}{\Ee{\textsf{X} \sim \varepsilon\br{\textsf{Y}}}{\ell\br{\textsf{Y},q\br{\textsf{X}}}}}$ we have that $\hat{\cR}_{\ell} \br{M,\eta,q} = \cR_{\ell} \br{\pi,\varepsilon,q}$ and $\underline{\hat{\cR}}_{\ell} \br{M,\eta} = \underline{\cR}_{\ell} \br{\pi,\varepsilon}$.
%	\item $\hat{\cR}_{\ell} \br{M,\eta,q} = \Ee{\textsf{X} \sim M}{L_\ell \br{\eta\br{\textsf{X}},q\br{\textsf{X}}}}$ and $\underline{\hat{\cR}}_{\ell} \br{M,\eta} = \Ee{\textsf{X} \sim M}{\underline{L}_\ell \br{\eta\br{\textsf{X}}}}$.
%	\item Since $\textcolor{orange}{\Ee{\br{\textsf{Y} , \textsf{X}} \sim D}{\tilde{\ell}\br{\textsf{Y},\tilde{q}\br{\textsf{X}}}} = \Ee{\textsf{X} \sim M}{\Ee{\textsf{Y} \sim \Pi_\Delta^{-1} \br{\tilde{\eta}\br{\textsf{X}}}}{\tilde{\ell}\br{\textsf{Y},\tilde{q}\br{\textsf{X}}}}} = \Ee{\textsf{Y} \sim \Pi_\Delta^{-1} \br{\tilde{\pi}}}{\Ee{\textsf{X} \sim \varepsilon\br{\textsf{Y}}}{\tilde{\ell}\br{\textsf{Y},\tilde{q}\br{\textsf{X}}}}}}$ we have that $\textcolor{orange}{\hat{\cR}_{\tilde{\ell}} \br{M,\tilde{\eta},\tilde{q}} = \cR_{\ell} \br{\tilde{\pi},\varepsilon,\tilde{q}}}$ and $\textcolor{orange}{\underline{\hat{\cR}}_{\tilde{\ell}} \br{M,\tilde{\eta}} = \underline{\cR}_{\tilde{\ell}} \br{\tilde{\pi},\varepsilon}}$.
%	\item $\textcolor{orange}{\hat{\cR}_{\tilde{\ell}} \br{M,\tilde{\eta},\tilde{q}} = \Ee{\textsf{X} \sim M}{L_{\tilde{\ell}} \br{\tilde{\eta}\br{\textsf{X}},\tilde{q}\br{\textsf{X}}}}}$ and $\textcolor{orange}{\underline{\hat{\cR}}_{\tilde{\ell}} \br{M,\tilde{\eta}} = \Ee{\textsf{X} \sim M}{\underline{L}_{\tilde{\ell}} \br{\tilde{\eta}\br{\textsf{X}}}}}$.
%\end{itemize}
%
%By replacing 
%\begin{itemize}
%	\item $\ell$ by $\Delta \ell$, we obtain $L_{\Delta \ell}$, $\textcolor{cyan}{\cR_{\textcolor{black}{\Delta \ell}}}$, $\cR_{\Delta \ell}$, $\underline{\cR}_{\Delta \ell}$, $\hat{\cR}_{\Delta \ell}$, and $\underline{\hat{\cR}}_{\Delta \ell}$.
%	\item $\textcolor{orange}{\tilde{\ell}}$ by $\textcolor{orange}{\Delta \tilde{\ell}}$, we obtain $\textcolor{orange}{L_{\Delta \tilde{\ell}}}$, $\textcolor{cyan}{\cR_{\textcolor{orange}{\Delta \tilde{\ell}}}}$, $\textcolor{orange}{\cR_{\Delta \tilde{\ell}}}$, $\textcolor{orange}{\underline{\cR}_{\Delta \tilde{\ell}}}$, $\textcolor{orange}{\hat{\cR}_{\Delta \tilde{\ell}}}$, and $\textcolor{orange}{\underline{\hat{\cR}}_{\Delta \tilde{\ell}}}$.
%	\item $\textcolor{red}{\ell}$ by $\textcolor{red}{\Delta \ell}$, we obtain $\textcolor{red}{L_{\Delta \ell}}$, $\textcolor{cyan}{\cR_{\textcolor{red}{\Delta \ell}}}$, $\textcolor{red}{\cR_{\Delta \ell}}$, and $\textcolor{red}{\underline{\cR}_{\Delta \ell}}$.
%	\item $\textcolor{violet}{\tilde{\ell}}$ by $\textcolor{violet}{\Delta \tilde{\ell}}$, we obtain $\textcolor{violet}{L_{\Delta \tilde{\ell}}}$, $\textcolor{cyan}{\cR_{\textcolor{violet}{\Delta \tilde{\ell}}}}$, $\textcolor{violet}{\cR_{\Delta \tilde{\ell}}}$, and  $\textcolor{violet}{\underline{\cR}_{\Delta \tilde{\ell}}}$.
%\end{itemize}
%
